# Supplementary material for: ProofWala: A Framework for Multilingual Proof Data Synthesis and Theorem-Proving
Source: arXiv:2502.04671 source file (2026-05-29)
Supplement: Supplementary file 1 [file appendix.tex]

\subsection{Training data for proof step prediction modules}
\label{app:training-data}
The training data is extracted in generic \texttt{JSON} format as shown in \Cref{fig:training-data-collection-format}. We create prompts to train the proof step generation model as demonstrated in \Cref{fig:prompt-format} from the collected raw data. 

\begin{figure}[H]
\begin{mdframed}[roundcorner=5pt]
\begin{minipage}{0.45\linewidth}
(a)
\begin{minted}[breaklines]{json}
{
"theorem_name": "nat_plus_0_is_n"
"start_goals": [
    {
        "hypotheses": [],
        "goal": "forall n : nat, n + 0 = n",
        "# ... extra metadata"
    }
],
"proof_steps": ["intros n."],
"end_goals": [
    {
        "hypotheses": ['n: nat'],
        "goal": "n + 0 = n",
        "# ... extra metadata"
    }
],
"# ... extra metadata"
} 
\end{minted}
\end{minipage}
\begin{minipage}{0.45\linewidth}
(b)
\begin{minted}[breaklines]{json}
{
"theorem_name": "nat_plus_0_is_n"
"start_goals": [
    {
        "hypotheses": [],
        "goal": "∀ (n : Nat), Nat.add n 0 = n",
        "# ... extra metadata"
    }
],
"proof_steps": ["intro n"],
"end_goals": [
    {
        "hypotheses": ['n : Nat'],
        "goal": "Nat.add n 0 = n",
        "# ... extra metadata"
    }
],
"# ... extra metadata"
} 
\end{minted}
\end{minipage}
\end{mdframed}
\caption{An excerpt from the extracted training data sequence, $\pi=\langle (O_0, a_1), \dots, (O_i, a_i), \dots (O_{n-1}, a_n)\rangle$ (see \Cref{sec:problem-formulation}), for a given theorem in \coq\; and \lean\; 4. The training data extracted here is used to train \proofwala\; proof step generation models. Here, $O_i$ i.e. set of obligations is extracted under \texttt{start\_goals} key while $O_{i+1}$ is represented under \texttt{end\_goals}. The action $a_i$ is extracted as the value of \texttt{proof\_steps} key. There are more fields other than the ones shown in the figure. (a) Shows an example of a Coq proof step, and (b) shows an example of a Lean proof step.}
\label{fig:training-data-collection-format}
\end{figure}

\begin{figure}[H]
\begin{mdframed}[roundcorner=5pt]
\begin{minipage}{0.5\linewidth}
\begin{minted}[breaklines]{md}
(a)
`Goals to prove:`
`[GOALS]`
`[GOAL] 1`
 S (n + 1) = S (S n)
`[HYPOTHESES] 1`
`[HYPOTHESIS]` IHn : n + 1 = 1 + n
`[HYPOTHESIS]` n : nat
`[END]`
\end{minted}
\begin{minted}[breaklines]{md}





(c)
`[RUN TACTIC]`
 auto.
`[END]`
\end{minted}
\end{minipage}
\begin{minipage}{0.5\linewidth}
(b)
\begin{minted}[escapeinside=||,mathescape=true,breaklines]{md}
`Goals to prove:`
`[GOALS]`
`[GOAL] 1`
 a + x ∈ [a + b-[|$\mathbb{K}$|]a + c] ↔ x ∈ [b-[|$\mathbb{K}$|]c]
`[HYPOTHESES] 1`
`[HYPOTHESIS]` |$\mathbb{K}$| : Type u_1
`...`
`[HYPOTHESIS]` π : ι → Type u_6
`[HYPOTHESIS]` inst✝⁵ : OrderedRing |$\mathbb{K}$|
`...`
`[HYPOTHESIS]` a x b c : E
`[END]`
\end{minted}
(d)
\begin{minted}[breaklines]{md}
`[RUN TACTIC]`
 simp [segment_eq_image']
`[END]`
\end{minted}
\end{minipage}
\end{mdframed}
\caption{Prompt format for training the proof step generation model. (a) shows the prompt format for \coq\;, (b) shows the prompt format for \lean\; 4, (c) shows the response format used for \coq, and (d) shows the response format used for \lean\; 4. We adopted a format similar to the one used in COPRA \cite{thakur2024incontext} but without any error context. It is important to note that we do not mention any information about the domain or ITP assistant in the prompt. The prompt format is the same for both languages.}
\label{fig:prompt-format}
\end{figure}

\section{ITP Versioning and Support}
\label{app:isabelle-support}

\paragraph{Version Compatibility.} Our framework supports multiple versions of Coq (v8.12–v8.18) and Lean 4 (v4.7.0-rc2 and v4.17.0), including those used in \texttt{MiniF2F} and other benchmarks. This flexibility is enabled through standardized JSON-based representations and a language-agnostic prompt format.

\paragraph{Isabelle Integration.} We also provide support for Isabelle via the PISA server, which offers a JSON-RPC interface for interaction. However, we did not conduct large-scale training or evaluation with Isabelle due to substantial system-level constraints. Each PISA instance requires a full copy of Isabelle and its heap images (∼35~GiB), which scales poorly in parallel settings (e.g., >1~TiB for 50 servers). In addition, memory usage per server can exceed 400~GiB, making distributed parallelism impractical on shared infrastructure. Unlike Lean’s lightweight REPL—which we optimized with custom restart logic—PISA is a heavyweight service, and similar fixes are nontrivial. Still, our interface abstractions and data formats already accommodate Isabelle, and future work may enable scalable experiments as tooling improves.

\subsection{Parallel Proof Search Beam Algorithm}
\label{app:parallel-proof-search}

\Cref{fig:beam-search-code} shows the parallel beam search pseudocode. We utilize the interface module's capabilities to create multiple instances of the proof environment and parallel run tactics to efficiently run search which can be scaled across nodes.

\newcommand{\Initialize}{\proc{Initialize}}
\newcommand{\GenerateProofSteps}{\proc{GenerateProofSteps}}

\newcommand{\Execute}{\proc{ExecuteParallel}}
\newcommand{\Timeout}{\mathit{t}}
\newcommand{\Model}{\mathit{model}}
\newcommand{\Width}{\mathit{width}}
\newcommand{\ItpInterface}{\proc{ItpInterface}}
\newcommand{\ItpInterfacePool}{\proc{ItpInterfacePool}}
\newcommand{\Pool}{\mathit{pool}}
\newcommand{\Frontier}{\mathit{frontier}}
\newcommand{\TimeElapsed}{\proc{TimeElapsed}}
\newcommand{\ProofTree}{\mathit{proof\_tree}}

\begin{figure}[H]
% \footnotesize
\begin{codebox}
\Procname{$\proc{ParallelBeamSearch}$($O_0$, $\Model$, $\Timeout$, $\Width$)}
\li \Comment{Set the pool of $\ItpInterface$ instances to state $O_{0}$} 
\li $\Pool \gets \ItpInterfacePool.\Initialize(O_{0})$
\li $\Frontier \gets \{O_{0}\}$
\li $\ProofTree \gets \phi$
\li \While $\Frontier \ne \phi$ 
\li \Do 
    \li \If $\TimeElapsed(\Timeout)$
            \li \Comment{Proof not found within the timeout}
            \li \Then \Return $\proc{False}$, $\ProofTree$
            \li \Else $\mathbb{O} \gets \phi$ \Comment{To store next possible states}
                \li \For $O \in \Frontier$
                \li \Do $\mathbb{A} \gets \GenerateProofSteps(O, \Model, \Width)$
                        \li \Comment{Filter a sub-pool from $\ItpInterface$ instances which are initialized to state $O$}
                        \li $\Pool' \gets \Pool.\proc{Filter}(O)$ 
                        \li \If $\Pool'$ is \textbf{empty}
                            \li \Then $\Pool' \gets \ItpInterfacePool.\Initialize(O)$
                            \li $\Pool.\proc{Merge}(\Pool')$ \Comment{Merge the new instances to the pool}
                        \End
                        \li \Comment{Execute generated possible proof step(s), $\mathbb{A}$, in parallel using the $\Pool'$}
                        \li $\mathbb{O} \gets \mathbb{O} \land \Pool'.\Execute(\mathbb{A})$
                        \li \Comment{Add all $\mathbb{A}$ edges in the $\ProofTree$ with $O$ as parent}
                        \li \If $\QED \in \mathbb{O}$
                                \li \Then \Return $\proc{True}$, $\ProofTree$
                            \End
                    \End
                \li $\Frontier \gets \mathbb{O}$
                \li \Comment{Filter the top $\Width$ states based on some heuristic}
                \li \Comment{for example log-likelihood of proof step leading to the state.}
                \li $\Frontier \gets \Frontier.\proc{TopK}(\Width)$
        \End
    \End
\End
\li \Return $\proc{False}$, $\ProofTree$
\end{codebox}
\caption{
Pseudocode for the parallel proof search module utilizing Beam Search with the Ray framework \cite{moritz2018ray}. This approach enables concurrent exploration of multiple proof steps (tactics) generated by the \proofwala\; model, improving efficiency and throughput. Unlike frameworks such as LeanDojo \cite{yang2023leandojo} for \lean\; 4, which operate sequentially, this module replicates instances of the \textbf{interface module} (see \Cref{sec:interface-module}) as a custom pool of Ray actors. The custom pool keeps track of ITP instances' proof state. It only uses those instances whose proof state matches the frontier state to continue the exploration (with the occasional overhead of adding more instances to the pool).  Each instance in the pool executes potential proof steps in parallel, allowing the search to proceed across various states simultaneously, avoiding the sequential overhead of executing steps one after another on the same ITP instance.
}
\label{fig:beam-search-code}
\end{figure}

\subsection{Hyperparameters used for training \proofwala\; models}
\label{app:hyperparams}

\begin{table}[ht]
    \centering
    \scalebox{0.7}{
    \begin{tabular}{ll}
    \hline
    \thead{\textbf{Hyperparameter}}  & \thead{\textbf{Value}}\\
    \toprule
    \textbf{Pretrained Model Name} & \codeTFive-\base\;(220 M) \\
    \textbf{Learning Rate} & $2 \times 10^{-4}$\\
    \textbf{Learning Scheduler Type} & \texttt{cosine}\\
    \textbf{Warmup Ratio} & \texttt{0.03}\\
    \textbf{Weight Decay} & \texttt{0.001}\\
    \textbf{Max Grad Norm (Gradient Clipping)} & \texttt{0.3}\\
    \textbf{Optimizer} & \texttt{adamw\_torch}\\
    \textbf{Gradient Accumulation Steps} & \texttt{1}\\
    \textbf{Max \# Steps (Gradient Updates)} & 34000\\
    \textbf{Batch Size} & 128\\
    \textbf{Checkpoint \# Steps} & 20000\\
    \textbf{Max \# Tokens} & 2048\\
    \bottomrule
    \end{tabular}}
    \caption{Hyperparameters used for training our \proofwala-\{\lean, \coq, \multi\}. In line with recent work on training multilingual models for autoformalization \cite{jiang2023multilingualmathematicalautoformalization}, we used the same step count and batch sizes to train all our models on different data mixes ensuring our ablation studies about the transfer were fair and were not merely a result of training more on bigger data-mixes.}
    \label{tab:hyperparams}
\end{table}

We trained our model in a distributed way via \textsc{PyTorch} and \textsc{HuggingFace} libraries. We used a cluster with 16 Nvidia \texttt{GH 200} GPU nodes to train \proofwala\; models. The training lasted for approximately 3 days. For further fine-tuning on CategoryTheory data we used the same parameters as shown in \Cref{tab:hyperparams}, except we ran only for 1200 steps with a smaller batch size of 8 (the checkpoint step was also accordingly reduced to 1200). Running all our training for various models for a fixed number of steps and the same batch size ensures that every model gets the same number of gradient updates. 

\subsection{Parameters used for proof search}
\label{app:search-params}

For all our experiments the beam width is 32 (see \Cref{tab:search-params}), and the temperature for the proof step prediction model is 0.75. We also have a timeout of 600 seconds for each proof attempt for all data mixes except GeoCoq where the timeout was 1200 seconds. Since the proofs in GeoCoq were long (sometimes more than 100 tactics), giving more time for the search to finish was important.

\begin{table}[ht]
    \centering
    \scalebox{0.7}{
    \begin{tabular}{ll}
    \hline
    \thead{\textbf{Parameter}}  & \thead{\textbf{Value}}\\
    \toprule
    \textbf{Search Algorithm} & Beam Search \\
    \textbf{Heuristic} & \thead[l]{Guided by \\Neg. Log-Likelihood \\of proof steps predicted \\by \proofwala\; models}\\
    \textbf{Beam Width} & \texttt{32}\\
    \textbf{Timeout} & \texttt{600} seconds\\
    \thead[l]{\textbf{\proofwala\;}\\\textbf{model Temp}} & 0.75\\
    \bottomrule
    \end{tabular}}
    \caption{Parameters used for searching for the complete proof using \proofwala\; models for guidance. We use beam search similar to GPT-$f$ \cite{polu2020generative}.}
    \label{tab:search-params}
\end{table}

\subsection{Bug Fixes in existing framework}
\label{app:bug-fixes}
Our framework built on top of \texttt{coq\_serapy}\footnote{\href{https://github.com/HazardousPeach/coq\_serapy}{https://github.com/HazardousPeach/coq\_serapy}} \cite{sanchez2020generating}, while our \lean\; 4 implementation is built on top of \texttt{REPL}\footnote{\href{https://github.com/leanprover-community/repl}{https://github.com/leanprover-community/repl}} library. We have enhanced these libraries by adding a common abstraction so that data can be collected across multiple languages. We also added ray actors \cite{moritz2018ray} to make it work across clusters on multiple machines. We also fixed some issues with these libraries, for example, \texttt{REPL} has a bug that allows it to accept incomplete and incorrect proofs\footnote{\href{https://github.com/leanprover-community/repl/issues/44}{https://github.com/leanprover-community/repl/issues/44}}.
We also fixed some memory issues which can arise when the REPL library keeps clones of proof-state to allow easy backtracking which leads to exponential memory increase. These fixes were essential for making the framework scalable and run on multiple nodes.

\subsection{Proof Tree annotations}
\label{app:proof-trees}

\Cref{fig:proof-search-annotation} shows a visualization generated using our tool. We can use these annotated trees to do qualitative analysis or train models for expert iteration.

\begin{figure}[H]
\centering
\footnotesize
\subfigure[]{\includegraphics[scale=0.3]{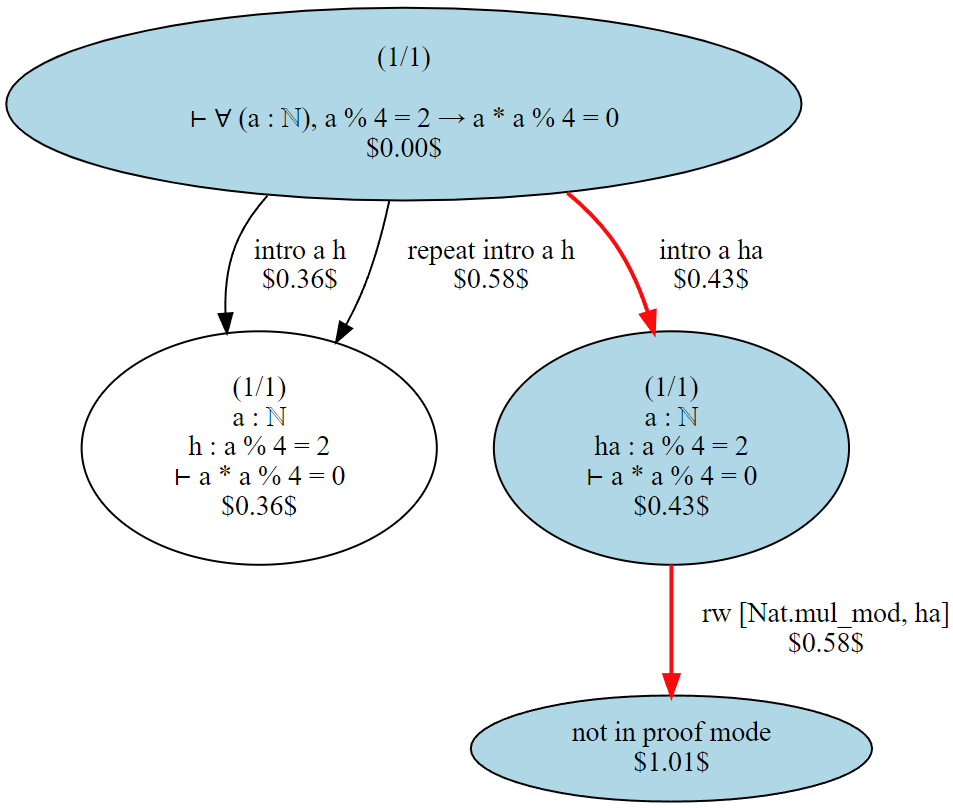}}\\
\subfigure[]{\includegraphics[scale=0.5]{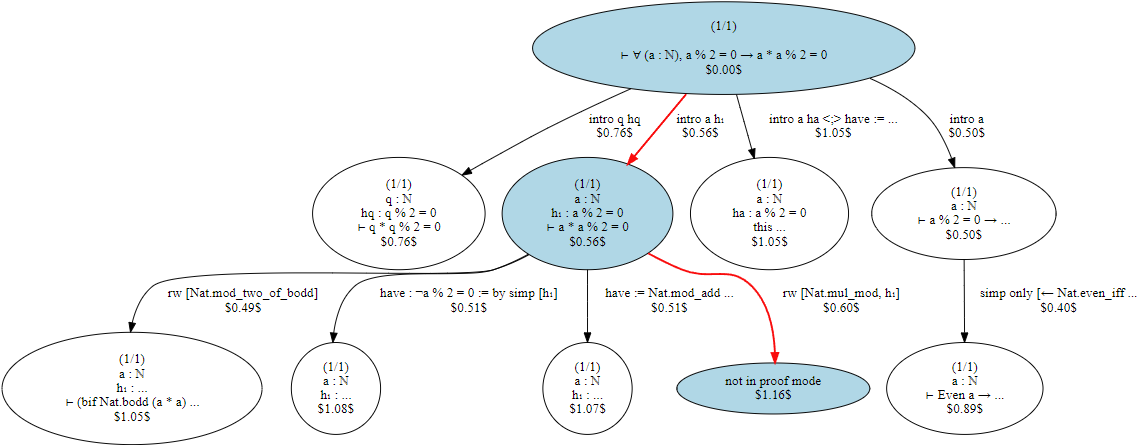}}
\caption{Visualization of the proof trees generated via the \textbf{Proof Search Module} (see \Cref{sec:searching-module}) for Lean 4 theorems stating: (a) \texttt{$\forall (a : \mathbb{N}), a\;\%\;4 = 2 \rightarrow a * a\; \%\;4 = 0$}, and (b) \texttt{$\forall (a : \mathbb{N}), a\;\%\;2 = 0 \rightarrow a * a\; \%\;2 = 0$}. The proof tree can be annotated with the correct proof path, and scores for each edge (proof step) and node (proof-state). This tree has been generated through Beam Search guided by the \proofwala-\multi\;model, the framework also supports best first search. The tree only includes proof steps (edges) that can be applied to the given proof-state (node) without any error. The numbers within the \$ symbols are the negative log-likelihood of the tokens generated by the \proofwala-\multi\; proof step generation model.}
\label{fig:proof-search-annotation}
\end{figure}

\section{Examples of Cross-Lingual Transfer in Category Theory}
\label{app:cat-theory-examples}

To better understand the cross-lingual transfer discussed in \Cref{sec:experiments}, we examined specific theorems in the Category Theory dataset. We identified Coq theorems that the multilingual model successfully proved, while the Coq-only model failed. For these cases, we found structurally analogous Lean theorems in the training data, particularly those involving categorical notions such as adjunctions, monicity, and currying.

\Cref{tab:cat-theory-transfer} shows representative examples. These qualitative results illustrate the model's ability to leverage shared categorical abstractions across ITPs and reinforce our hypothesis about effective structural transfer.

\begin{table}[h]
\centering

\begin{tabular}{|p{4.2cm}|p{7.0cm}|c|c|}
\hline
\textbf{Coq Theorem} & \textbf{Lean 4 Equivalent} & \textbf{Multilingual} & \textbf{Coq-Only} \\
\hline
\texttt{counit\_fmap\_unit} \newline $\forall\; x,\; \varepsilon \circ \mathsf{fmap}[F]\; \eta \approx \mathsf{id}[F(x)]$
& \texttt{adjointify\_$\eta$\_$\varepsilon$ (X : C)} \newline 
$F.\mathsf{map}((\mathsf{adjointify}_{\eta, \varepsilon}).\mathsf{hom.app}(X)) \gg \varepsilon.\mathsf{hom.app}(F.\mathsf{obj}(X)) = \mathbb{1}(F.\mathsf{obj}(X))$
& \ding{51} & \ding{55} \\
\hline
\texttt{id\_monic} \newline $\forall\; x,\; \mathsf{Monic}(\mathsf{id}_{x})$
& \texttt{cancel\_mono\_id (f : X -> Y)} \newline 
$g \gg f = f \;\Leftrightarrow\; g = \mathbb{1}_X$
& \ding{51} & \ding{55} \\
\hline
\texttt{eval\_first} \newline $\mathsf{eval} \circ \mathsf{first}(f) \approx \mathsf{uncurry}(f)$
& \texttt{uncurry\_id\_eq\_ev (A X : C)} \newline $\mathsf{uncurry}(\mathbb{1}_{A \Rightarrow X}) = (\mathsf{exp.ev}(A)).\mathsf{app}(X)$
& \ding{51} & \ding{55} \\
\hline
\end{tabular}
\caption{Examples of Category Theory theorems in Coq and their Lean equivalents. The multilingual model succeeds, while the Coq-only model fails.}
\label{tab:cat-theory-transfer}
\end{table}

\subsection{Qualitative Analysis: Proof Tree Properties}
\label{app:proof-tree-properties}

Across various data mixes we observe that proof trees found using the \multi\; model tend to have more nodes, edges, and higher degrees per node (see \Cref{tab:tree-stats}). \Cref{fig:proof-tree-stats-nodes}, \Cref{fig:proof-tree-stats-edges}, and \Cref{fig:high-degree} show the distribution of nodes, edges, and degrees respectively. \Cref{fig:proof-tree-stats-same-proof} shows that \multi\; often found more proofs for the same theorem during the search.

% \begin{wraptable}{l}{0.6\textwidth}
% \vspace{-0.25in}
\begin{table}[H]
    \centering
    \scalebox{1.0}{
    \begin{tabular}{lllllllll}
    \toprule
    \textbf{Data-Mix} &  
    \textbf{\name Model} &
    \multicolumn{3}{c}{\textbf{Avg. Proof Tree Stats}} &
    \\
    \cmidrule(lr){3-5}
     & 
     & 
    \textbf{\# Nodes} &
    \textbf{\# Edges} & 
    \textbf{\# Degree} \\
    \toprule
    \textbf{\lean} & 
    \lean & 
     {3.989} & 
     {3.536} & 
     {1.536}
    \\
     & 
     \multi & 
    4.729 & 
    4.689 & 
    1.983
    \\
    \hline
    \textbf{MathComp} & 
    \coq & 
    2.534 & 
    1.739 & 
    1.167
    \\
     &
     \multi & 
     2.576 & 
     1.822 & 
     1.207 
     \\
    \hline
    \textbf{GeoCoq} & 
    \coq & 
     15.358 & 
     14.457 & 
     1.180
    \\
    & 
    \multi & 
     17.144 & 
     15.75 & 
     1.353
    \\
    \hline
    \textbf{CompCert} &
    \coq &  
     8.048 & 
     7.480 & 
     1.404 
     \\
     &
     \multi & 
     8.318 & 
     8.200 & 
     1.584 
     \\
    \hline
    \textbf{CategoryTheory} & 
    \coq-\CatTheory & 
    5.674 & 
    5.804 & 
    2.301 
    \\
    & 
    \multi-\CatTheory & 
    7.056 & 
    7.130 & 
    2.193
    \\
    \bottomrule
    \end{tabular}}
    \caption{Comparison between the average number of nodes, edges, and degree of the proof trees generated on various \proofwala$\;$models over different data-mixes.}
    \label{tab:tree-stats}
\end{table}
% \end{wraptable}

%================= PROOF TIME TABLE (Avg Only) =================
\begin{table}[ht]
\centering
\begin{tabular}{llr}
\toprule
\textbf{Data Mix} & \textbf{\name\; Model} & \textbf{Avg} \\
\midrule
\lean    & \multi & 30.5296 \\
         & \lean  & 20.7370 \\
\midrule
CompCert & \multi & 59.9424 \\
         & \coq   & 70.3282 \\
\midrule
MathComp & \multi & 8.9993  \\
         & \coq   & 7.5634  \\
\midrule
GeoCoq   & \multi & 107.1999 \\
         & \coq   & 74.3914  \\
\midrule
CategoryTheory & \multi & 39.2182 \\
               & \coq   & 27.4105 \\
\bottomrule
\end{tabular}
\caption{Summary of \emph{average} proof times (in seconds) across various data mixes. We can see that \name-\multi\; usually searches for longer and hence the average time is higher. Since the proof trees generated are larger for \multi\; approach, it is reasonable that overall proof search time will be higher.}
\label{tab:app-proof-times-avg}
\end{table}

We observe that \multi\; model usually searches longer for proofs across the different data mixes. The average time taken to search for proof is summarized in the \Cref{tab:app-proof-times-avg} and the distribution of proof search time is shown in \Cref{fig:proof-tree-stats-time}.

%================= PROOF LENGTH TABLE (Avg Only) =================
\begin{table}[ht]
\centering
\begin{tabular}{llr}
\toprule
\textbf{Data Mix} & \textbf{\name\; Model} & \textbf{Avg} \\
\midrule
\lean      & \multi & 2.0363 \\
           & \lean  & 2.0679 \\
\midrule
CompCert   & \multi & 4.7913 \\
           & \coq   & 5.0270 \\
\midrule
MathComp   & \multi & 2.4940 \\
           & \coq   & 2.4759 \\
\midrule
GeoCoq     & \multi & 9.2486 \\
           & \coq   & 10.6954 \\
\midrule
CategoryTheory & \multi & 3.4909 \\
               & \coq   & 3.0426 \\
\bottomrule
\end{tabular}
\caption{Summary of \emph{average} proof lengths across various data mixes. The proof lengths are not very different for the two approaches.}
\label{tab:app-proof-lengths-avg}
\end{table}

Interestingly, we see that there is no significant difference in the size of the proof (number of tactics used) found via the two approaches. \Cref{tab:app-proof-lengths-avg} summarizes the length of the proofs found during the search.

\begin{figure}[H]
\footnotesize
\includegraphics[scale=.3]{img-node-distribution.png}
\caption{Distribution of proof-tree nodes across various data-mixes found by different \name\; models. It is interesting to note that across all data-mixes, the \name-\multi\; model tends to produce more nodes per proof tree. This indicates that \name-\multi\; often constructs larger proof trees during search.}
\label{fig:proof-tree-stats-nodes}
\end{figure}

\begin{figure}[H]
\footnotesize
\includegraphics[scale=0.3]{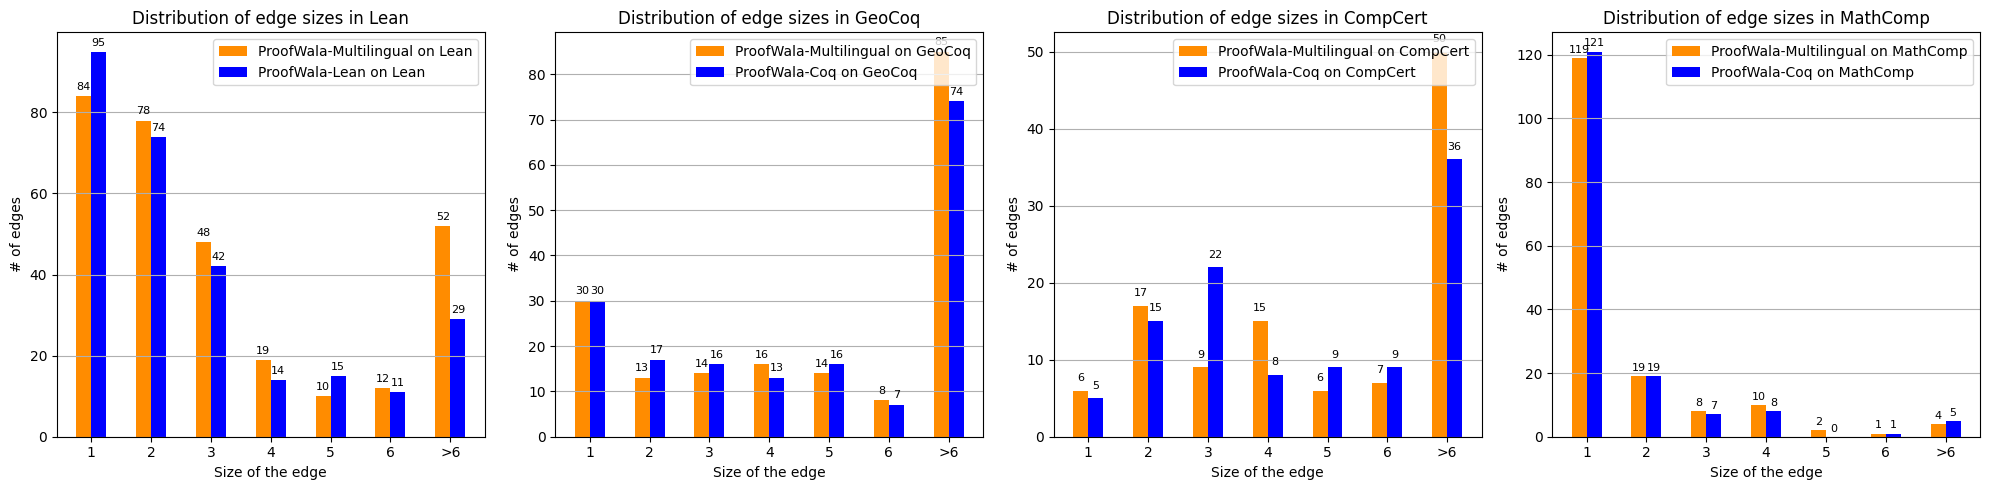}
\caption{Distribution of proof-tree edges across various data-mixes found by different \name\; models. It is interesting to note that across all data mixes, \name-\multi\; models tend to have more edges per proof tree. This indicates that \name-\multi\; often find more compilable tactics while searching to complete the proof.}
\label{fig:proof-tree-stats-edges}
\end{figure}

\begin{figure}[H]
\footnotesize
\includegraphics[scale=0.3]{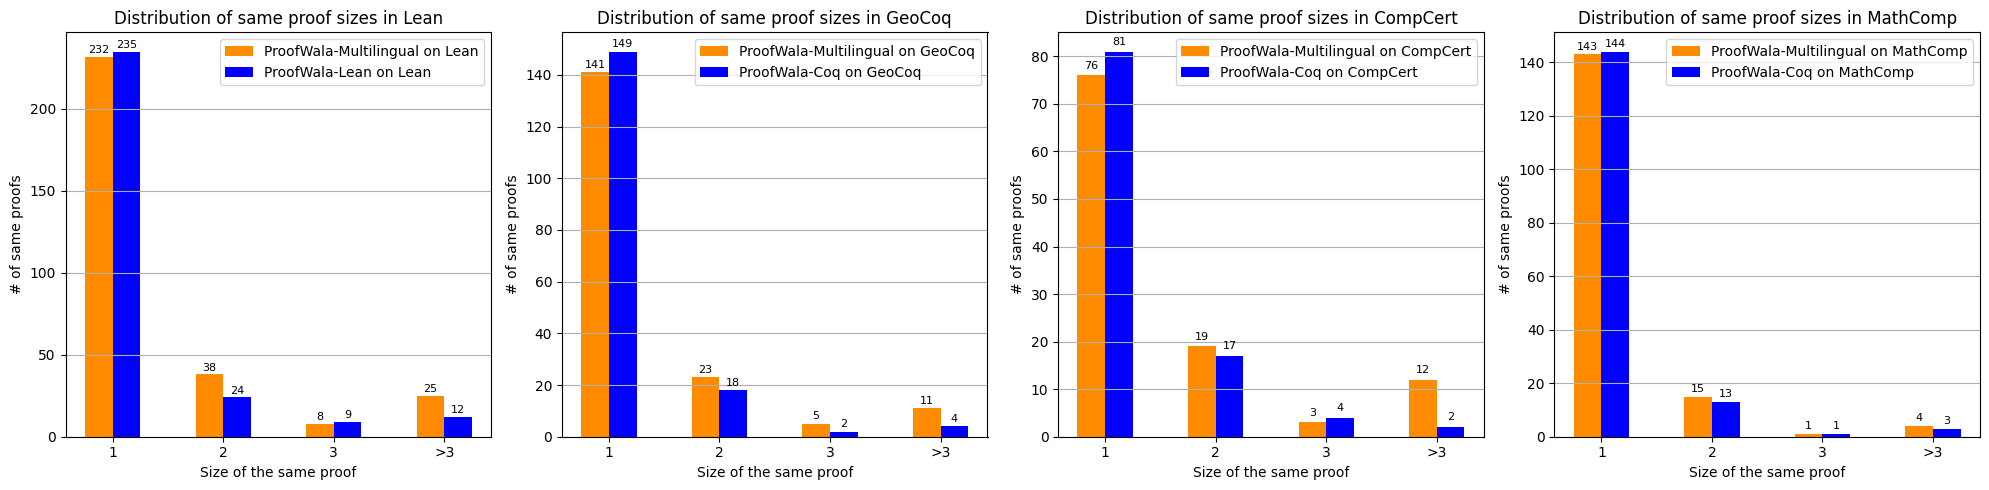}
\caption{Distribution of the number of proofs found for the same theorem across various data-mixes found by different \name\; models. It is interesting to note that across all data mixes, the \name-\multi\; model tends to produce more proofs for the same theorem.}
\label{fig:proof-tree-stats-same-proof}
\end{figure}

\begin{figure}[H]
\footnotesize
\includegraphics[scale=0.3]{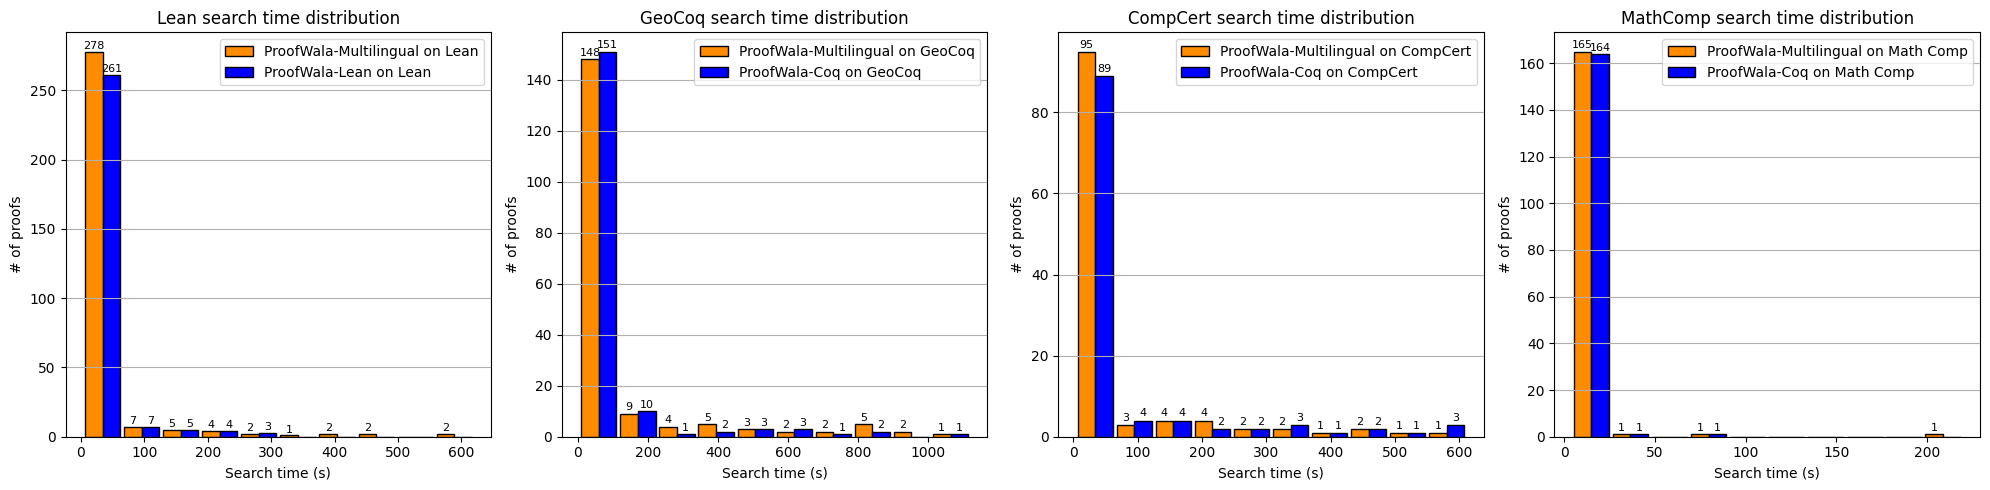}
\caption{Distribution of the time taken to find proofs across various data-mixes found by different \name\; models. We can see that across all data mixes, the \name-\multi\; model tend to run longer proof searches, and thus effectively search more.}
\label{fig:proof-tree-stats-time}
\end{figure}

\subsection{Qualitative Analysis: Proofs found by \multi\; model}
\label{app:proofs}

\Cref{fig:app-example-lean} shows some of the \lean{} 4 and \coq{} proofs found by \multi{} model.

\begin{figure}[H]
%\vspace{-0.1in}
\begin{mdframed}[roundcorner=10pt]
(a)
\begin{minipage}{0.9\textwidth}
\begin{lstlisting}
theorem lapMatrix_toLin'_apply_eq_zero_iff_forall_reachable (x : V → ℝ) :
    Matrix.toLin' (G.lapMatrix ℝ) x = 0 ↔ ∀ i j : V, G.Reachable i j → x i = x j  := by
    rw [← (posSemidef_lapMatrix ℝ G).toLinearMap₂'_zero_iff, star_trivial,
        lapMatrix_toLinearMap₂'_apply'_eq_zero_iff_forall_adj]
    refine ⟨?_, fun h i j hA ↦ h i j hA.reachable⟩
    intro h i j ⟨w⟩
    induction' w with w i j _ hA _ h'
    rfl
    exact (h i j hA).trans h'
\end{lstlisting}
\end{minipage}
\\(b)
\begin{minipage}{0.9\textwidth}
\begin{lstlisting}
theorem interval_average_symm (f : ℝ → E) (a b : ℝ) : (⨍ x in a..b, f x) = ⨍ x in b..a, f x  := by
    simp only [intervalIntegral, setAverage_eq, smul_sub]
    obtain rfl | hab := eq_or_ne a b
    rfl
    rw [uIoc_comm a b, uIoc_comm b a]
\end{lstlisting}
\end{minipage}
\\(c)
\begin{minipage}{0.9\textwidth}
\begin{minted}[breaklines]{Coq}
Theorem coplanar_perm_11  : forall A B C D,
  Coplanar A B C D -> Coplanar B D C A.
Proof.
    intros A B C D HCop.
    destruct HCop as [X H]; exists X.
    induction H; try (induction H); spliter; Col5.
Qed.
\end{minted}
\end{minipage}
\\(d)
\begin{minipage}{0.9\textwidth}
\begin{minted}[breaklines]{Coq}
Theorem coprimepP: forall  p q , 
 reflect (forall d, d %| p -> d %| q -> d %= 1) (coprimep p q).
Proof.
    rewrite /coprimep; apply: (iffP idP) => [/eqP hs d dvddp dvddq | h].
    have/dvdp_eqp1: d %| gcdp p q by rewrite dvdp_gcd dvddp dvddq.
    by rewrite -size_poly_eq1 hs; exact.
    by rewrite size_poly_eq1; case/andP: (dvdp_gcdlr p q); apply: h.
Qed.
\end{minted}
\end{minipage}
\end{mdframed}
%\reducevspacebetweenfigureandcaption
\vspace{-0.1in}
\caption{Some proofs discovered by \proofwala-\multi\; in our experiments on theorems from Mathlib, GeoCoq, and MathComp.}
\label{fig:app-example-lean}
\end{figure}
